# Supplementary material for: Computing Teichm\"{u}ller Maps between Polygons
Source: arXiv:1401.6395 source file (2014-01-24)
Supplement: Supplementary file 1 [file appendix2.tex]

\section{Complete proofs of theorems}
\seclabel{app2}

\latertextnow
