# Supplementary material for: Computing Teichm\"{u}ller Maps between Polygons
Source: arXiv:1401.6395 source file (2014-01-24)
Supplement: Supplementary file 2 [file appendix3.tex]

\section{Detailed simulations}
\seclabel{app3}
